# Supplementary material for: Sketch and Project: Randomized Iterative Methods for Linear Systems and Inverting Matrices
Source: arXiv:1612.06013 source file (2016-12-19)
Supplement: Supplementary file 1 [file appendix_template.tex]

%---------------------------------------------------------------------------------
%	APPENDIX One (J. Miocic template)
%---------------------------------------------------------------------------------
\chapter[Appendix 1]{All the material that didn't make it into the thesis}
\chaptermark{Appendix A}
\label{ch:AppendixA} % label for referring to chapter in other parts of the thesis
\textbf{ABSTRACT}\\
\small{Chapter abstract} % Having a chapter abstract is optional
\vfill
\small{\textbf{Author Contributions:} During long nights postgraduate A compiled this appendix}
\newpage
\section[Stuff related to Chapter 1]{Sadly there is a word limit of 70,000 in the main thesis :-()}
\subsection{Stuff} \label{A1:Stuff}
